# Supplementary material for: SigOpt Mulch: An Intelligent System for AutoML of Gradient Boosted Trees
Source: arXiv:2307.04849 source file (2023-07-10)
Supplement: Supplementary file 1 [file appendix.tex]

\section{Metalearning}\label{sec:appendix_metalearning}

\textbf{Training datasets:}
'australian', 'bands', 'biodegredation', 'breast-cancer', 'default-credit', 'dow-jones-index', 'eeg-eye-state', 'german-numeric', 'hill\_valley', 'magic04', 'mammographic\_masses', 'parkinsons', 'spambase', 'tic-tac-toe', 'transfusion', 'wdbc', 'wholesale'

\noindent \textbf{Testing datasets:}
'haberman', 'relax', 'sonar', 'pima-indians-diabetes'

\subsection{Parameter Importance}\label{sec:appendix_parameter_importance}

\begin{table}[ht]
\begin{tabular}{lr}
\toprule
{} &         0 \\
\midrule
eta              &  0.608877 \\
gamma            &  0.032165 \\
max\_depth        &  0.026800 \\
min\_child\_weight &  0.022148 \\
num\_boost\_round  &  0.016457 \\
\bottomrule
\end{tabular}
\caption{Average parameter importance in FANOVA testing\label{tab:fanova_mean}}
\end{table}

\begin{table*}
\begin{tabular}{lrrrrr}
\toprule
{} &       eta &     gamma &  max\_depth &  min\_child\_weight &  num\_boost\_round \\
\midrule
australian            &  0.883778 &  0.002586 &   0.001031 &          0.006589 &         0.005115 \\
bands                 &  0.742665 &  0.029423 &   0.051843 &          0.015703 &         0.003205 \\
biodegredation        &  0.620584 &  0.004765 &   0.020300 &          0.023807 &         0.018321 \\
breast-cancer         &  0.632665 &  0.011771 &   0.002993 &          0.015128 &         0.021870 \\
default-credit        &  0.322237 &  0.081587 &   0.016206 &          0.007865 &         0.007834 \\
dow-jones-index       &  0.824355 &  0.009368 &   0.007414 &          0.010490 &         0.020394 \\
eeg-eye-state         &  0.822370 &  0.003361 &   0.079586 &          0.002471 &         0.004913 \\
german-numeric        &  0.802104 &  0.015900 &   0.005087 &          0.014991 &         0.011037 \\
haberman              &  0.244209 &  0.199163 &   0.007991 &          0.025173 &         0.010621 \\
hill\_valley           &  0.218114 &  0.047442 &   0.122724 &          0.033700 &         0.022490 \\
magic04               &  0.734275 &  0.010606 &   0.031073 &          0.004777 &         0.002071 \\
mammographic\_masses   &  0.628249 &  0.009107 &   0.016772 &          0.013977 &         0.016166 \\
parkinsons            &  0.383583 &  0.023889 &   0.006017 &          0.127588 &         0.029400 \\
pima-indians-diabetes &  0.506394 &  0.011143 &   0.010599 &          0.018558 &         0.062303 \\
relax                 &  0.210463 &  0.133584 &   0.017251 &          0.019282 &         0.038642 \\
sonar                 &  0.835312 &  0.007907 &   0.005793 &          0.019605 &         0.002200 \\
spambase              &  0.807453 &  0.002215 &   0.014477 &          0.004083 &         0.008750 \\
tic-tac-toe           &  0.694966 &  0.003102 &   0.130998 &          0.001963 &         0.017185 \\
transfusion           &  0.425560 &  0.054170 &   0.007289 &          0.058796 &         0.006251 \\
wdbc                  &  0.700124 &  0.004105 &   0.003452 &          0.018891 &         0.032865 \\
wholesale             &  0.746962 &  0.010275 &   0.003908 &          0.021678 &         0.003958 \\
\bottomrule
\end{tabular}
\caption{Parameter importance by training dataset for FANOVA testing \label{tab:fanova_all}}
\end{table*}

\subsection{Few Shot Learning: Prior estimation}\label{sec:appendix_FSL}

This section details the prior estimation techniques mentioned in  Section  \ref{sec:few_shot_learning}. Let us denote by $\{\theta_i\}_{i=1}^n$ the top configurations by resulting metric after aggregating an equal number of top configurations from each dataset. The development in this paper was done for the accuracy metric, but the techniques are easily transferable to other metrics. Assuming \eqref{eq:density_decomp} holds, fitting to overall density $\varrho$ amounts to fitting independent parameter densities $\varrho_j$ for $j=1,\dots,d$.

To fit a uniform density to $\{\theta_i\}_{i=1}^n$, we search for bounds $L_j$ and $U_j$ for independent uniforms $\mathcal{U}(L_j,U_j)$ across $j=1,\dots,d$. Taking independent quantiles proved to be a simple, performant, and flexible method for deriving such bounds. Specifically, for $j=1,\dots,d$ we set $L_j$ as the $\underline{q}_j$-quantile and $U_j$ as the $\overline{q}_j$-quantile of single parameter configurations $\{\theta_{ij}\}_{i=1}^n$. Settings for pairs $(\underline{q}_j,\overline{q}_j)$ were derived based on the authors' experience and knowledge of GBT. 

The authors compared a variety of non-uniform fits using SciPy's distributions and built in support for maximum likelihood estimation of distribution parameters. The best fits, shown in Figure \ref{fig:densities}, were chosen because they captured data trends in $\{\theta_{ij}\}_{i=1}^n$ and/or biased towards more performant settings.

\section{Cost awareness}
\subsection{Correlation, Precision and Recall Scores}
\label{sec:correlation_precision_recall}
\textbf{Definitions.} We state rigorous mathematical definition of the correlation, precision and recall scores here. Let $X = \{x_1, \dots, x_m\}$ be a set of hyperparameter configurations, and let $Y_p = \{y^i_p\}_{i=1}^{m}$ be a list of GBT accuracy evaluated at $X$ and a fidelity $p$. 
Let $\tilde{Y}_p$ be the normalized accuracy, i.e. $\tilde{Y}_p = \{(y^i_p - y_{\min})/(y_{\max} - y_{\min}) \}_{i=1}^{m}$. 
For a low fidelity $p_0$ and the highest fidelity $p_1 = 1$, we use the following three scores to quantify the similarity between $Y_{p_0}$ and $Y_{p_1}$.
First, we define the \textit{correlation score} of $Y_{p_0}$, denoted $S_{correlation}(Y_{p_0})$ as the Pearson correlation computed from $Y_{p_0}$ and $Y_{p_1}$. 
Second, we define the \textit{precision score} of $Y_{p_0}$ as
$$
S_{precision}(Y_{p_0}) = \frac{1}{|\mathcal{I}_0|} \sum_{i \in \mathcal{I}_0} \tilde{y}^i_{p_1},
$$
where $\mathcal{I}_0$ contains $X$ indices corresponding to the top $10$-th percentile of $Y_{p_0}$.

$$
S_{recall}(Y_{p_0}) = \frac{1}{|\mathcal{I}_1|} \sum_{i \in \mathcal{I}_1} \tilde{y}^i_{p_0},
$$
where $\mathcal{I}_1$ contains $X$ indices corresponding to the top $10$-th percentile of $Y_{p_1}$.

\textbf{Detailed scores for all datasets.} For each of the 23 balanced binary datasets, we present the detailed correlation, precision and recall scores in \tabref{table:all scores 1} and \tabref{table:all scores 2}.
 
\section{Empirical Studies}

This section details the empirical studies  touched on in \secref{sec:ES}. 

% The XGB-MF algorithm is detailed in Algorithm \ref{algo:XGB-MF}. 

% \newpage
% \begin{figure*}[ht]
%     \includegraphics[width=0.75\linewidth]{figs/violins.pdf}
%     \centering
%     \caption{Each violin shows the distribution of best accuracies found after 8 initial samples from a variety of initial sampling schemes. The violins are overlayed onto the distribution of optimal accuracies found by repeatedly running BO out to \AGSNote{\#} iterations. \AGSNote{needs updating!}}
%     \label{fig:violins}
% \end{figure*}

% \newpage
\begin{table}[]
\caption{Detailed correlation, precision and recall scores for each dataset. \label{table:all scores 1}}
% \small
\tabcolsep 3pt
\begin{tabular}{lrrrr}
\toprule
dataset& \multicolumn{1}{l}{p} & \multicolumn{1}{l}{Correlation} & \multicolumn{1}{l}{Precision} & \multicolumn{1}{l}{Recall} \\ \hline
adult & 0.1 & 0.64   & 0.98 & 0.97     \\
    & 0.3 & 0.70  & 0.98 & 0.97     \\
    & 0.5 & 0.68   & 0.98 & 0.97     \\
    & 0.7 & 0.69   & 0.98 & 0.97     \\ \hline
australian     & 0.1 & 0.86   & 0.93 & 0.92     \\
    & 0.3 & 0.92   & 0.94 & 0.97     \\
    & 0.5 & 0.92   & 0.94 & 0.96     \\
    & 0.7 & 0.92   & 0.94 & 0.95     \\  \hline
bands  & 0.1 & 0.40   & 0.81 & 0.76     \\
    & 0.3 & 0.82   & 0.86 & 0.90     \\
    & 0.5 & 0.86   & 0.88 & 0.88     \\
    & 0.7 & 0.87   & 0.87 & 0.91     \\ \hline
biodegredation & 0.1 & 0.74   & 0.92 & 0.95     \\
    & 0.3 & 0.78   & 0.93 & 0.96     \\
    & 0.5 & 0.77   & 0.91 & 0.97     \\
    & 0.7 & 0.79   & 0.94 & 0.96     \\ \hline
breast-cancer  & 0.1 & 0.51   & 0.90 & 0.93     \\
    & 0.3 & 0.83   & 0.93 & 0.94     \\
    & 0.5 & 0.87   & 0.94 & 0.93     \\
    & 0.7 & 0.88   & 0.93 & 0.95     \\ \hline
default-credit & 0.1 & 0.49   & 0.98 & 0.93     \\
    & 0.3 & 0.57   & 0.98 & 0.93     \\
    & 0.5 & 0.56   & 0.98 & 0.94     \\
    & 0.7 & 0.55   & 0.98 & 0.94     \\ \hline
dow-jones-index& 0.1 & 0.84   & 0.88 & 0.95     \\
    & 0.3 & 0.93   & 0.89 & 0.96     \\
    & 0.5 & 0.94   & 0.93 & 0.96     \\
    & 0.7 & 0.92   & 0.89 & 0.97     \\ \hline
eeg-eye-state  & 0.1 & 0.96   & 0.96 & 0.90     \\
    & 0.3 & 0.98   & 0.96 & 0.91     \\
    & 0.5 & 0.98   & 0.95 & 0.92     \\
    & 0.7 & 0.98   & 0.95 & 0.93     \\ \hline
german-numeric & 0.1 & 0.38   & 0.98 & 0.80     \\
    & 0.3 & 0.72   & 0.99 & 0.97     \\
    & 0.5 & 0.71   & 0.99 & 0.97     \\
    & 0.7 & 0.72   & 0.99 & 0.97     \\ \hline
haberman& 0.1 & 0.31   & 0.86 & 0.93     \\
    & 0.3 & 0.27   & 0.86 & 0.88     \\
    & 0.5 & 0.29   & 0.87 & 0.83     \\
    & 0.7 & 0.37   & 0.87 & 0.90     \\ \hline
heart  & 0.1 & 0.14   & 0.93 & 0.42     \\
    & 0.3 & 0.77   & 0.92 & 0.78     \\
    & 0.5 & 0.81   & 0.93 & 0.81     \\
    & 0.7 & 0.85   & 0.93 & 0.86     \\ \hline
hill\_valley   & 0.1 & -0.07  & 0.28 & 0.56     \\
    & 0.3 & -0.06  & 0.41 & 0.21     \\
    & 0.5 & 0.08   & 0.35 & 0.52     \\
    & 0.7 & -0.08  & 0.35 & 0.52     \\ \hline
magic04& 0.1 & 0.84   & 0.96 & 0.95     \\
    & 0.3 & 0.85   & 0.96 & 0.95     \\
    & 0.5 & 0.85   & 0.97 & 0.94     \\
    & 0.7 & 0.84   & 0.96 & 0.95     \\ \hline
mammographic\_masses  & 0.1 & 0.86   & 0.96 & 0.92     \\
    & 0.3 & 0.87   & 0.96 & 0.96     \\
    & 0.5 & 0.88   & 0.96 & 0.96     \\
    & 0.7 & 0.89   & 0.96 & 0.95     \\ \hline
\end{tabular}
\end{table}

% \newpage
\begin{table}[]
\caption{Detailed correlation, precision and recall scores for each dataset. \label{table:all scores 2}}
% \small
\tabcolsep 3pt
\begin{tabular}{lrrrr}
\toprule
dataset& \multicolumn{1}{l}{p} & \multicolumn{1}{l}{Correlation} & \multicolumn{1}{l}{Precision} & \multicolumn{1}{l}{Recall} \\ \hline
parkinsons     & 0.1 & 0.40   & 0.83 & 0.95     \\
    & 0.3 & 0.50   & 0.89 & 0.88     \\
    & 0.5 & 0.59   & 0.89 & 0.88     \\
    & 0.7 & 0.63   & 0.89 & 0.89     \\ \hline
pima-indians-diabetes & 0.1 & 0.57   & 0.88 & 0.87     \\
    & 0.3 & 0.75   & 0.88 & 0.93     \\
    & 0.5 & 0.74   & 0.88 & 0.93     \\
    & 0.7 & 0.69   & 0.88 & 0.91     \\ \hline
relax  & 0.1 & 0.18   & 0.75 & 0.90     \\
    & 0.3 & 0.24   & 0.77 & 0.90     \\
    & 0.5 & 0.24   & 0.83 & 0.79     \\
    & 0.7 & 0.27   & 0.84 & 0.80     \\ \hline
sonar  & 0.1 & 0.05   & 0.49 & 0.19     \\
    & 0.3 & 0.71   & 0.80 & 0.85     \\
    & 0.5 & 0.73   & 0.82 & 0.87     \\
    & 0.7 & 0.81   & 0.80 & 0.86     \\ \hline
spambase& 0.1 & 0.86   & 0.97 & 0.93     \\
    & 0.3 & 0.87   & 0.96 & 0.94     \\
    & 0.5 & 0.89   & 0.95 & 0.95     \\
    & 0.7 & 0.88   & 0.96 & 0.94     \\ \hline
tic-tac-toe    & 0.1 & 0.68   & 0.97 & 0.79     \\
    & 0.3 & 0.70   & 0.98 & 0.70     \\
    & 0.5 & 0.79   & 0.98 & 0.78     \\
    & 0.7 & 0.84   & 0.97 & 0.83     \\ \hline
transfusion    & 0.1 & 0.43   & 0.91 & 0.96     \\
    & 0.3 & 0.44   & 0.91 & 0.92     \\
    & 0.5 & 0.38   & 0.91 & 0.94     \\
    & 0.7 & 0.41   & 0.92 & 0.93     \\ \hline
wdbc& 0.1 & 0.64   & 0.95 & 0.90     \\
    & 0.3 & 0.82   & 0.95 & 0.95     \\
    & 0.5 & 0.85   & 0.96 & 0.95     \\
    & 0.7 & 0.86   & 0.96 & 0.93     \\ \hline
wholesale      & 0.1 & 0.32   & 0.92 & 0.78     \\
    & 0.3 & 0.79   & 0.93 & 0.97     \\
    & 0.5 & 0.78   & 0.93 & 0.97     \\
    & 0.7 & 0.82   & 0.93 & 0.96     \\ \hline
\end{tabular}

\end{table}

\begin{figure*}[ht!]
    \includegraphics[trim={0 1.5cm 0 0},clip, width=\textwidth]{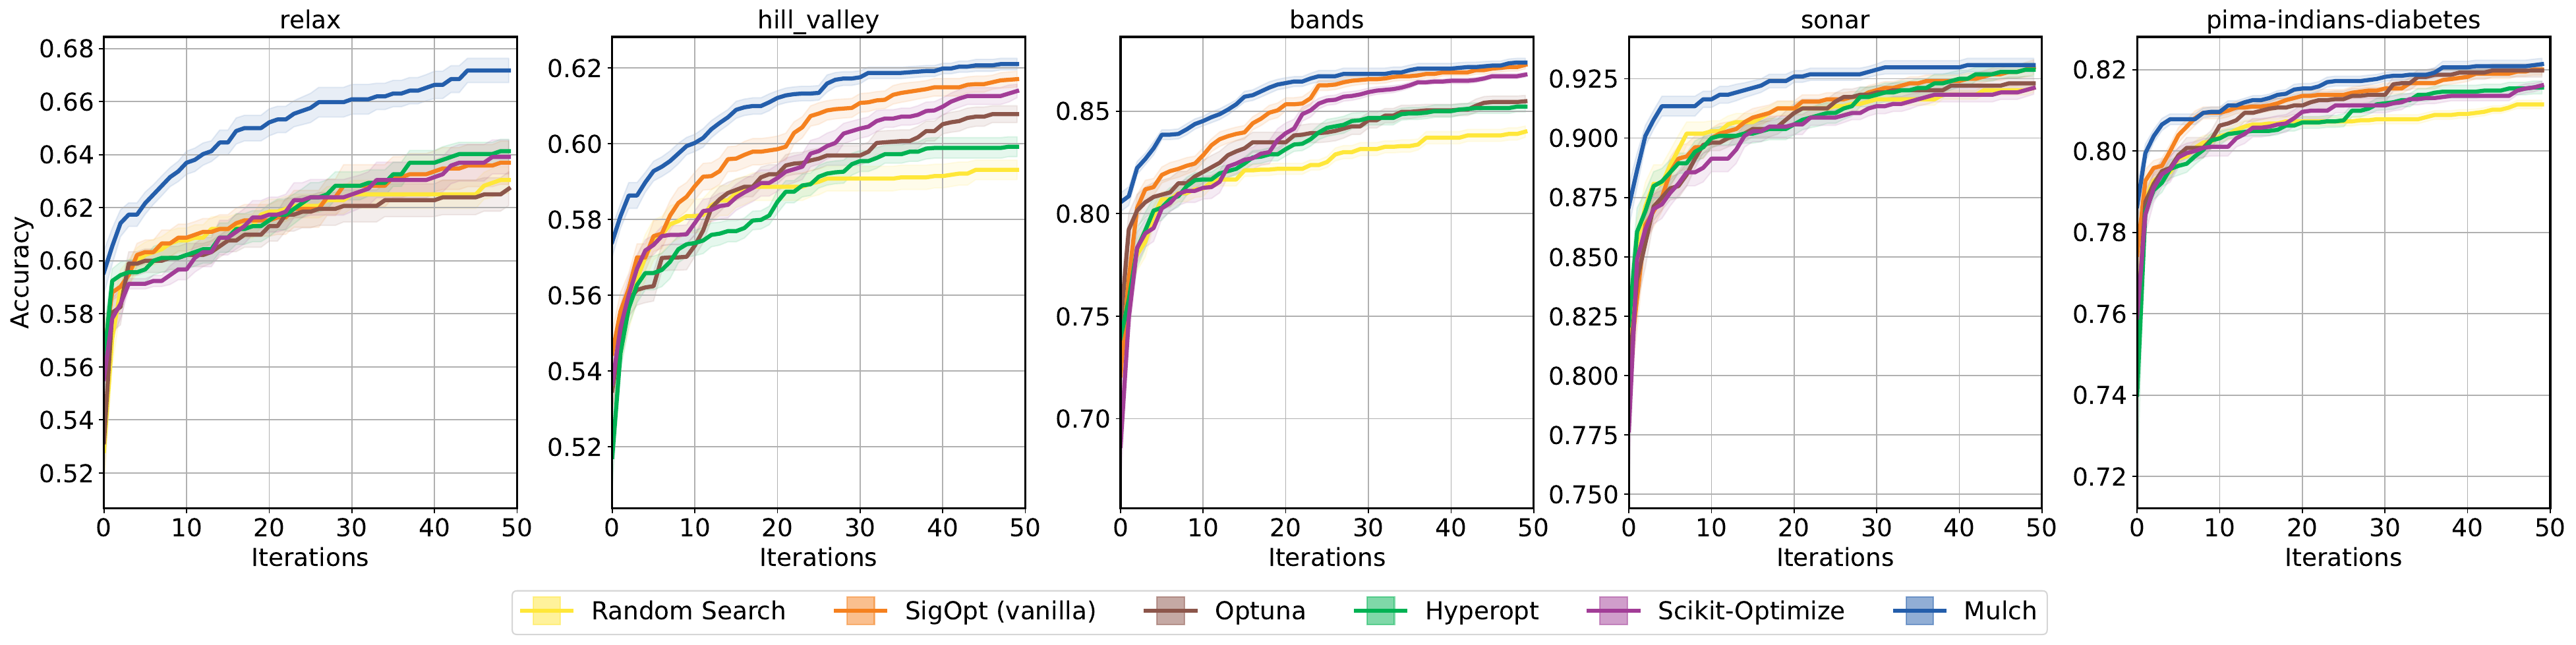}
    \includegraphics[width=\textwidth]{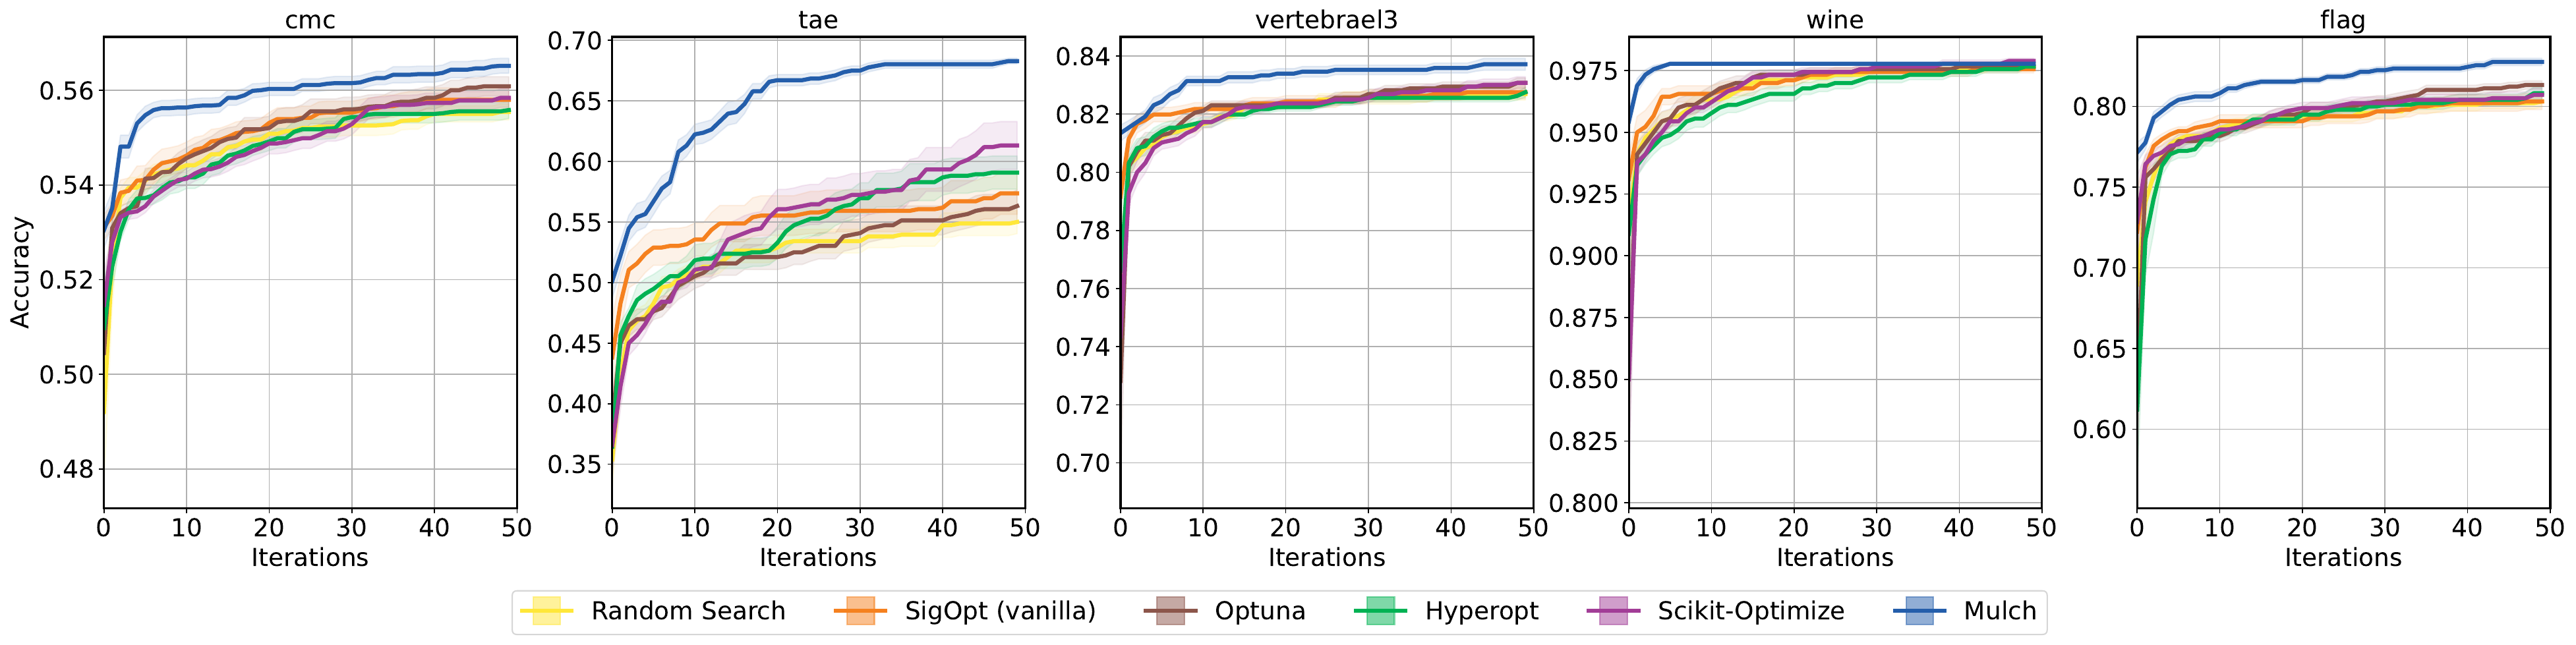}
    \centering
    \caption{Mulch's metalearning (blue) results in identification of better models compared to: vanilla SigOpt (orange), Optuna (black), Hyperopt (green), Scikit-optimize (purple), and random search (yellow). In this case, we are benchmarking Mulch on a set ten unseen classification problems, and measuring model performance through classification accuracy.}
    \label{fig:warmstart_full_bo_runs_multiclass}
\end{figure*}
